# Supplementary material for: Graph Neural Processes for Spatio-Temporal Extrapolation
Source: arXiv:2305.18719 source file (2023-05-30)
Supplement: Supplementary file 1 [file appendix.tex]

\section{Mathematical Notation}
\label{sec:notation}
We define the major mathematical notations in the paper in Table~\ref{table_notation} for better understanding. 
\begin{table}[!h]
\centering
\caption{Major notations used in the paper.}
\label{table_notation}

  \begin{threeparttable}
  \begin{tabular}[width=0.69\linewidth]{lll}
    \toprule
      Notation & Dimension & Description \\
      \midrule
    $N$, $M$ & $\mathbb{R}^1$ & number of context, target nodes\\
    $T$ & $\mathbb{R}^1$ & time length of a sequence\\ 
    $A_{m,n}$ & $\mathbb{R}^1$ & weight between node $m$ and $n$\\
    $n$, $m$  & $\mathbb{R}^1$ & index of a context and target node\\
    $d_l$, $d_x$, $d_y$ & $\mathbb{R}^1$ & feature dimensionalities\\
    \midrule
    $\mathcal{C}$ & $\mathbb{R}^{N\times T\times (d_x+d_y)}$ & context set\\
    $\mathcal{D}$ & $\mathbb{R}^{M\times T\times (d_x+d_y)}$ & target set\\
    $H$ & $\mathbb{R}^{M\times T\times \sum_{l=1}^Ld_l)}$ & representations of all context nodes\\
    \midrule
    $A$ & $\mathbb{R}^{M\times N}$ & adjacency matrix \\
    $X_n$, $Y_n$ & $\mathbb{R}^{T\times (d_x+d_y)}$ & covariates, data of a context node\\
    $X_m$, $Y_m$ & $\mathbb{R}^{T\times (d_x+d_y)}$ &  those of a target node\\
    $H_n$ & $\mathbb{R}^{T\times \sum_{l=1}^Ld_l}$ &  representations of context node $n$\\
    $V_m$ & $\mathbb{R}^{T\times \sum_{l=1}^Ld_l}$ & representations of target node $m$\\
    $R_n$ & $\mathbb{R}^{T\times \sum_{l=1}^Ld_l}$ & latent observations of node $n$\\
    $Z_m$ & $\mathbb{R}^{T\times \sum_{l=1}^Ld_l}$ & latent variables of target node $m$\\
    \midrule
    $x_{n,t}$, $y_{n,t}$ & $\mathbb{R}^{d_x+d_y}$ & data of context node $n$ at time $t$\\
    $h_{i,t}$ & $\mathbb{R}^{\sum_{l=1}^Ld_l}$ & representation of node $i$ at time $t$\\
  \bottomrule
\end{tabular}
\end{threeparttable}
\end{table}

\section{Derivation of Graph Bayesian Aggregation}
\label{sec:deriGBA}
In this section, we give formal derivations of the proposed Graph Bayesian Aggregation. We first derive the general GBA without factorization or specific graph stricture. We assume a latent prior $Z$ over a target node (omitting subscript $m$ for brevity). The latent observation functions of all context nodes are an independent linear transformation of $Z$ following Gaussian distributions: 
\begin{align}
&p(Z)=\mathcal{N}(Z|\mu,\Lambda^{-1}),\\
&p(R_n|Z)=\mathcal{N}(R_n|A_n Z,L_n^{-1})\quad\text{  For } n \in [1, N],
\end{align}
where we use the precision matrix $\Lambda$ and $L$ for convenience; $A_n$ is a transformation matrix, representing the graph structure. The logarithmic joint probability over $Z$ and $[R_1, .., R_N]$ is:

\begin{eqnarray}    \label{eq}
\ln{p(Z, R_1, .., R_N)}&=&\ln{p(Z)}+\ln{p(R_{1} ...R_{N}|Z)}    \\
~&=&\ln{p(Z)} + \sum_{n=1}^{N} \ln{p(R_{n}|Z) } \nonumber    \\
~&=&-\frac{1}{2} (Z-\mu )^T\Lambda(Z-\mu)\nonumber\\
~&&\quad-\frac{1}{2}\sum_{n=1}^{N}(R_{i}-A_iZ)^TL_{i}(R_i-A_iZ)+\operatorname{Const}. \nonumber
\end{eqnarray}
We find the second term can be written as:
\begin{eqnarray}    \label{eq}
&&-\frac{1}{2}Z^\top(\Lambda+\sum_{n=1}^{N}A_{n}^\top L_{n}A_{n})Z \\
&&\qquad-\frac{1}{2}\sum_{n=1}^{N}R_{n}^\top L_{n}R_{n}
+\frac{1}{2}R_{n}^\top L_{n}A_{n}Z+\frac{1}{2}Z^\top A_{n}^\top L_{n}R_{n} \nonumber \\
&=&-\frac{1}{2}\begin{bmatrix}
    Z\\
    R_{1}\\
    \vdots \\
R_{N}
\end{bmatrix} 
\underbrace{
\begin{bmatrix}
    \Lambda+\sum_{n=1}^{N}A_{n}^{T}L_{n}A_{n} &  -A_{1}^{T}L_{1}&  \cdots & -A_{N}^{T}L_{N}\\
    -L_{1}A_{1}&  L_{1}&  \cdots & 0\\
    \vdots &  \vdots&  \ddots & \vdots \\
    -L_{N}A_{N}&  0&  \cdots& L_{N}
\end{bmatrix}
}_{P}
\begin{bmatrix}
    Z\\
    R_{1}\\
    \vdots\\
R_{N}\nonumber
\end{bmatrix}
\end{eqnarray}
According to~\cite{bishop2006pattern}, we notate $P$ as the precision matrix of the joint distribution. The covariance matrix is:
\begin{equation}
    \operatorname{cov}[Z, R_1, .., R_N]= P^{-1}
\end{equation}
Next, the linear terms reveal hints of the mean which are:
\begin{equation}
Z^\top\Lambda \mu = \begin{bmatrix}
Z\\
R_{1}\\
\vdots\\
R_{N}
\end{bmatrix}^\top\begin{bmatrix}
\Lambda \mu\\
0\\
\vdots\\
0
\end{bmatrix}
\end{equation}
Then, from~\cite{bishop2006pattern}, the mean is given by:
\begin{eqnarray}    \label{eq}
\mathbb{E}[Z, R_1, .., R_N] &=& P^{-1}\begin{bmatrix} 
    \Lambda \mu\\
    0\\
    \vdots\\
0
\end{bmatrix}
=\begin{bmatrix}
    \mu\\
    A_{1} \mu\\
    \vdots \\
A_{N} \mu
\end{bmatrix}
\end{eqnarray}
The mean and covariance of the marginal distribution of $p(R_1, .., R_N)$ can be calculated as:
\begin{equation}
E\begin{bmatrix}
    R_{1}&\cdots  &R_{N}
  \end{bmatrix}^\top=\begin{bmatrix}
   A_{1} \mu\\
  \vdots\\
  A_{N}\mu
  \end{bmatrix}
\end{equation}
 
\begin{equation}
Cov[R_{1} \cdots R_{N}] = \begin{bmatrix}
L_{1}^{-1} + A_{1}\Lambda^{-1} A_1^\top\\
\vdots\\
L_{N}^{-1} + A_{N}\Lambda^{-1} A_{N}^\top
\end{bmatrix}
\end{equation}
In the end, using Gaussian conditioning, we could obtain the probability of $p(z|R_1, .., R_N)$ which is also a Gaussian:
\begin{equation}
    {\textstyle \sum_{Z|R_{1}\cdots R_{N}}}=\left(L + \sum_{n=1}^{N}A_{n}\Lambda A_{n}^\top\right)^{-1} 
\end{equation}

\begin{eqnarray}    \label{eq}
\mu_{z|R_{1}\cdots R_{N}}&=&{\textstyle \sum_{z|R_{1}\cdots R_{N}}}\left ((\Lambda + \sum_{n=1}^{N}A_{n}^{T}L_{n}A_{n})\mu\right. \nonumber\\
&& \qquad \left.+\begin{bmatrix}A_{1}^{T}L,\cdots,A_{N}^{T}L\end{bmatrix}\left(\begin{bmatrix}
    R_{1}\\
    \vdots\\
R_{N}
\end{bmatrix}-\begin{bmatrix}
    A_{1}\mu\\
    \vdots\\
A_{N}\mu
\end{bmatrix}\right)  \right )   \nonumber    \\
&=&{\textstyle \sum_{z|R_{1}\cdots R_{N}}}\left( \Lambda \mu + \sum_{n=1}^{N}A_{n}^TL_{n}R_{n}  \right) 
\end{eqnarray}
As the Gaussian distributions are assumed to be factorized: $\Lambda^{-1}=\operatorname{diag}(\sigma_z)$ and $L_n^{-1}=\operatorname{diag}(\sigma_{R_n})$. The transformation $A_i=I(a_n)$ represents a scale distance weight $a_n$ between the target node and the context node $n$ in the adjacency matrix. Given these assumptions, the Gaussian can be further factorized as:
\begin{align}
    &\bar{\sigma}_{Z}^{2}=\left[\left(\sigma_{Z}\right)^{-2}+\sum_{n=1}^{N}\left( \sigma_{R_n} / a_n\right)^{-2}\right]^{-1}\\
    &\bar{\mu}_{Z}=\bar{\sigma}_{Z}^{2} \left( \mu_{Z} / \sigma^2_{Z} + \sum_{n=1}^{N} a_n R_{n} / \sigma^2_{R_n} \right)
\end{align}

\section{Derivation of ELBO for STGNP}
\label{sec:elbo}
In this section, we derive the evidence lower-bound (ELBO) for our STGNP.
\begin{align}
\begin{split}
    &\log p\left(Y_m \mid X_m, \mathcal{C}, A\right)\\
    &=\log \mathbb{E}_{q\left(Z \mid \mathcal{C}\cup \mathcal{D}, A\right)}\frac{p\left(Y_m, Z_m \mid X_m, \mathcal{C}, A\right)}{q\left(Z_m \mid \mathcal{C}\cup \mathcal{D}, A\right)}\\
    &\geq \mathbb{E}_{q\left(Z \mid \mathcal{C}\cup \mathcal{D}, A\right)} \left[ \log \frac{p\left(Y_m, z_m \mid Z_m, \mathcal{C}, A\right)}{q\left(X_m \mid \mathcal{C}\cup \mathcal{D}, A\right)} \right]\\
    &= \mathbb{E}_{q\left(Z_m \mid \mathcal{C}\cup \mathcal{D}, A\right)} \left[ \log \frac{
    p\left(Y_m \mid X_m, Z_m\right) p\left(Z_m \mid X_m, \mathcal{C}, A\right)}
    {q\left(Z_m \mid \mathcal{C}\cup \mathcal{D}, A\right)} \right]\\
    &= \mathbb{E}_{q\left(Z_m \mid \mathcal{C}\cup \mathcal{D}, A\right)} \left[ \log p\left(Y_m \mid X_m, Z_m\right)\right] 
    \\& \qquad\qquad - \mathbb{E}_{q\left(Z_m \mid \mathcal{C}\cup \mathcal{D}, A\right)} \left[ \log \frac{q\left(Z_m \mid \mathcal{C}\cup \mathcal{D}, A\right)}{p\left(Z_m \mid X_m, \mathcal{C}, A\right)} \right]\\
    &= \mathbb{E}_{q\left(Z_m \mid \mathcal{C}\cup \mathcal{D}, A\right)} \left[ \log p\left(Y_m \mid X_m, Z_m\right)\right] \\
    &\qquad\qquad- \mathbb{E}_{q\left(Z_m \mid \mathcal{C}\cup \mathcal{D}, A\right)} \left[ \log \frac{\prod_{l=1}^{L} q\left(Z^l_m \mid Z_m^{l+1}, {V^\prime}^l_m, H^l, A\right)}{\prod_{l=1}^{L} q\left(z_m^l \mid Z_m^{l+1}, V^l_m, H^l, A\right)} \right]\\
    &= \mathbb{E}_{q\left(Z_m \mid \mathcal{C}\cup \mathcal{D}, A\right)} \left[ \log p\left(Y_m \mid X_m, Z_m\right)\right] \\
    &-\sum_{l=1}^L \mathbb{E}_{q(Z_m^{l+1})} \left[\mathbb{KL}\left(q(Z_m^{l}|Z_m^{l+1}, {V^\prime}^l_m, H^l, A)||q(Z_m^l|Z_m^{l+1}, V^l_m, H^l, A)\right)\right].\\
\end{split}
\end{align}

\section{Experimental Details}
\subsection{Dataset Description}
\label{sec:dataset}
\begin{itemize}[leftmargin=*]
\item \textbf{Beijing}~\cite{zheng2015forecasting} The Beijing AQI dataset is an air quality index dataset collected from 36 stations (Station ID 1001-1036) in Beijing from May 1, 2014 to April 30, 2015. It includes six air quality attributes (i.e., concentrations of PM2.5, PM10, O3, NO2, SO2, and CO in micrograms per cubic meter) and district-level meteorological attributes (i.e., temperature, humidity, pressure, wind speed, direction, and weather). All signals are recorded hourly. %Following~\cite{cheng2018neural}, we use meteorological information to extrapolate PM2.5, PM10, and NO2. 
Note that we drop station 1022 due to its significant missing data.
\item \textbf{London}\footnote{\url{https://www.biendata.xyz/competition/kdd_2018/}} To evaluate the performance on other domains, we use the London AQI dataset~\cite{patel2022accurate}, which consists of data collected from 24 AQI stations in London from January 1, 2017 to March 31, 2018. It includes concentrations of PM2.5, PM10, and NO2 in micrograms per cubic meter and meteorological features recorded in a grid. To obtain the meteorological features for each AQI station, we take the average of the nearest four grid points, following~\cite{patel2022accurate}.
%Following~\cite{cheng2018neural}, we utilize meteorological attributes to infer air quality indexes.
\item \textbf{Water} The water dataset is an urban water quality dataset~\cite{liu2020predicting} reported from 15 water quality monitoring stations in Shenzhen City. It consists of 3 water measures residual chlorine (RC), turbidity (TU), and pH. We use TU and pH to extrapolate RC, as it is the most important measure for urban water systems. The data was collected every 5 minutes over a period of more than three years starting in 2011, but for this study, we only use data in 2012.
%The data is gathered every 5 minutes. The duration is more than 3 years since 2011 while we only employ data in 2012.
\end{itemize}

For NNs models, data preprocessing is utilized to fill in the missing values in the dataset. We adopt linear interpolation for numerical data and nearest interpolation for categorical features.
The adjacency matrix is constructed by longitudes and latitudes of stations and is normalized by a Gaussian kernel: $A_{m,n}=\exp(-\frac{dist(v_m, v_n)^2}{\sigma^2})$, where $\sigma$ is the standard deviation. $dist(v_m, v_n)$ is calculated by the Haversine formula.
\begin{align}
\begin{split}
    dist(v_i, v_j) &=2 r \arcsin \left(\sin ^{2}\left(\frac{\varphi_{j}-\varphi_{i}}{2}\right)+ \right.\\
    &\left.\cos \left(\varphi_{i}\right) \cos \left(\varphi_{j}\right) \sin ^{2}\left(\frac{\lambda_{j}-\lambda_{i}}{2}\right)\right)^{\frac{1}{2}},
\end{split}
\end{align}
where $r=6371 km$ is the radius of the earth, $(\varphi_{i}, \lambda_{i})$ means the longitude and latitude of a sensor $v_i$.

\subsection{Baseline Implementation Details} 
\label{sec:baselines}
\begin{itemize}[leftmargin=*]
\item \textbf{ANCL}~\cite{patel2022accurate} is a scalable method for air quality inference that uses non-stationary Gaussian processes. It includes a Hamming distance kernel and a locally periodic kernel to capture categorical and temporal features, respectively. The final predictions are a combination of all of the kernels, and the hyperparameters of these kernels, such as the length scale, are optimized using stochastic gradient descent.
\item \textbf{ADAIN}~\cite{cheng2018neural} is an attention-based neural network for data inference. For each node, it divides features into temporal and static parts and utilizes an MLP and RNN to encode them, separately. Then, an attention mechanism is leveraged to aggregate information from all nodes and generates the outputs. Here, we regard longitude and latitude as static features, and others as dynamic features.
\item \textbf{MCAM}~\cite{hanfine} is a multi-channel attention model for air quality inference. It learns separate adjacency matrices for static and dynamic features. Then, GCNs are leveraged to learn spatial relations for features of two kinds. In the end, fully-connected layers integrate information and obtain the output results. 
%It learns a static and dynamic adjacency matrix using the proposed attention mechanisms. The GNNs are adopted to obtain the output results. To construct dynamic adjacency, MCAM utilizes horizontal and vertical wind velocity so that they can only apply to air quality data, limiting its applicability.
\item \textbf{SGNP} is a variant of Sequential Neural Processes (SNP)~\cite{singh2019sequential} that combines both stochastic and deterministic parts to generate results. As SNP cannot handle the graph data, we have modified it by adding our cross-set graph neural network. In order to ensure a fair comparison, we have not used the posterior dropout training strategy introduced by SNP to alleviate the transition collapse problem, but this strategy can easily be applied to STGNP as well.
\item \textbf{SGANP} following the SNP's attentive variant~\cite{qin2019recurrent}, we also adopt an attentive version of SGNP. In particular, we replace CSGCN in the deterministic part of SGNP with an attention mechanism and the stochastic part remains the same.
\end{itemize}

For ANCL and other statistical methods, we adopt codes~\footnote{\url{https://github.com/patel-zeel/AAAI22}} released by the ANCL's authors. The rest neural network baselines are reimplemented by us according to their TensorFlow version code ~\footnote{\url{https://github.com/singhgautam/snp}} or their papers (ADAIN, MCAM). All hyperparameter settings are the same in their papers. It's worth noting that both ADAIN and MCAM use covariates such as point of interest (POI) and road network data, which are not publicly available. Therefore, in our experiments, we do not use these additional features. 

\subsection{STGNP Architectures}
\begin{figure}[!h]
  \centering
  \includegraphics[width=1\linewidth]{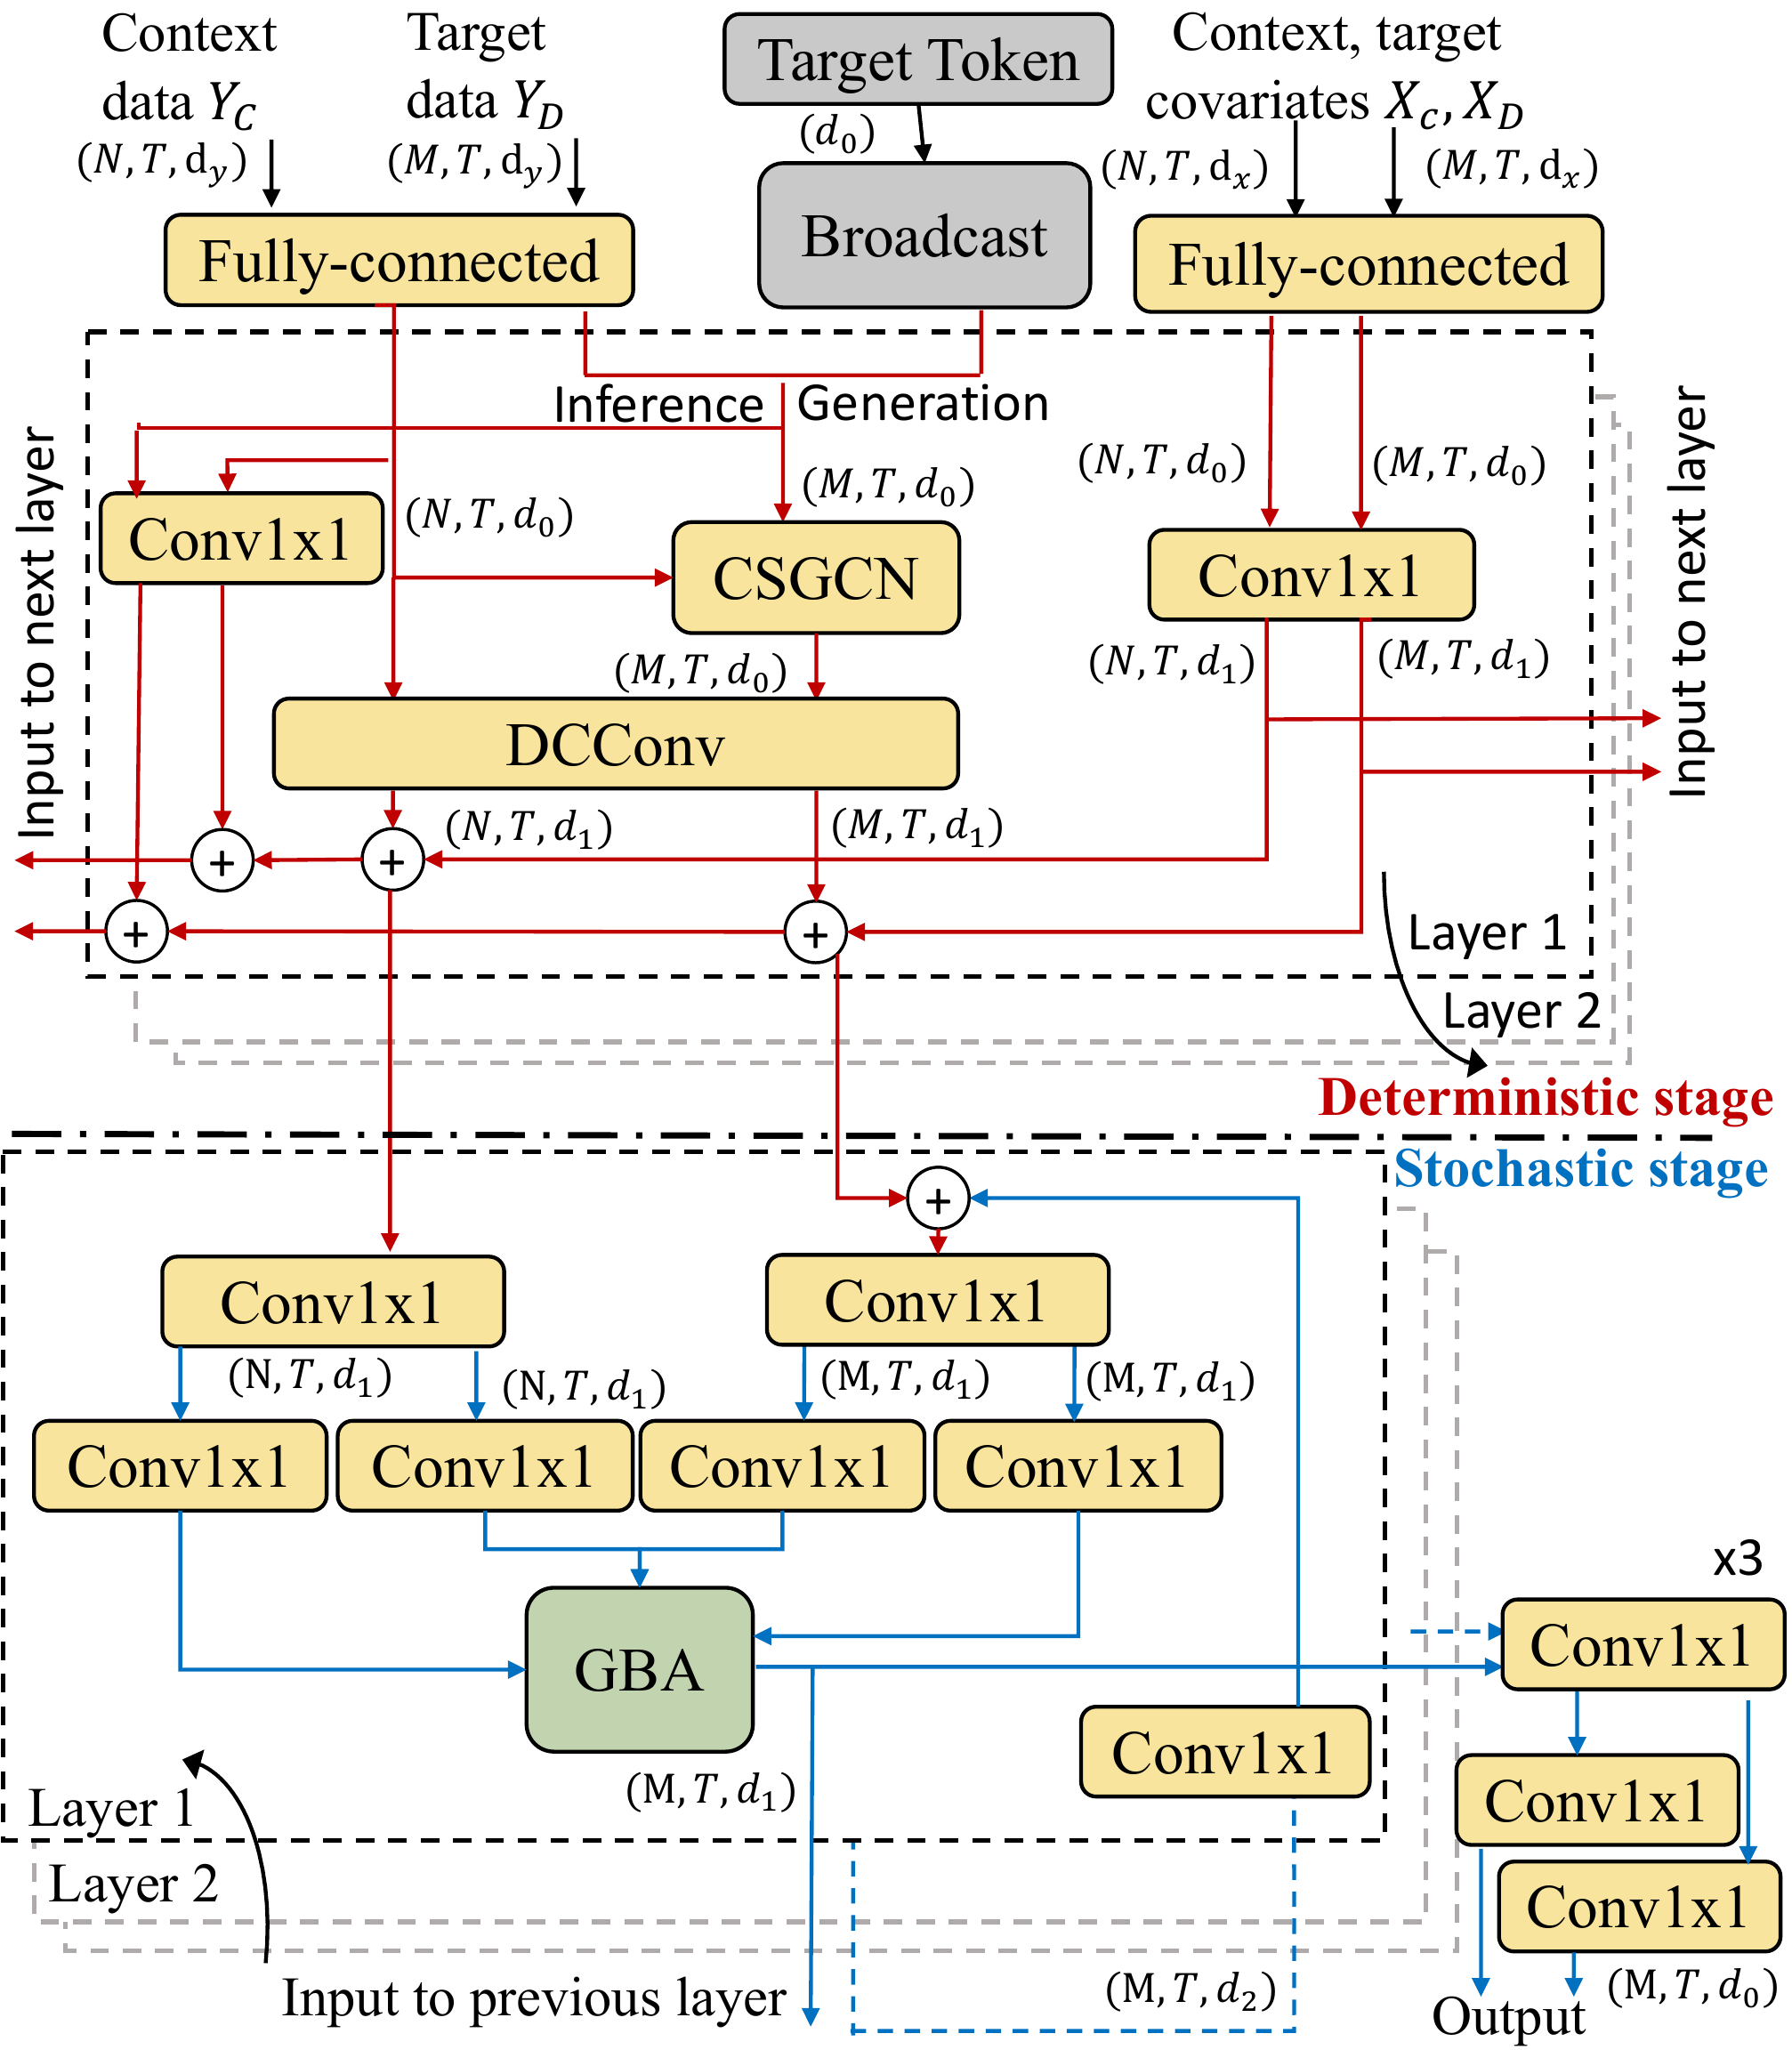}
  \caption{Architecture of STGNP for spatio-temporal extrapolation.}
\label{fig:arch}
\end{figure}

\label{sec:arch}
Our STGNP has two major architectural components for deterministic and stochastic learning as shown in Figure~\ref{fig:arch}:
\begin{itemize}[leftmargin=*]
\item \textbf{Deterministic spatio-temporal stage:} The core component of this stage is the spatio-temporal learning module consisting of dilated causal convolutions and cross-set graph neural networks. Each layer contains a CSGCN to learn spatial dependencies and a DCconv to model temporal relations of sensor data. At the first layer, features of covariates learned by another DCConv are added to the representations.
The convolution has a kernel size of $k=3$ and the number of output channels is denoted as $d$. The DCConv has a multilayer perceptron layer with $d$ neurons. We stack 3 layers with skip connections to capture spatial-temporal dependencies with $d=[16,32,64]$. The dilation factor is set to have an exponentially increasing rate of $2$ w.r.t the block so that we achieve a receptive field of $15$. Although this field is smaller than the length of the sequence ($T=24$), the ablation study shows that it still produces satisfactory performance.

\item \textbf{Stochastic generation stage:} The Graph Bayesian Aggregation and the likelihood function are chief modules. The GBA includes a module for the latent observation function which is a $1$-layer $1\times 1$ convolution with $d$ kernels, followed by 2 convolutions to obtain mean and variance. The prior has the same structure as the observation function, except it further takes an input sample from the next layer's posterior.
We stack $4$ GBAs corresponding to the $4$ blocks in the first stage with $d=[16, 32, 64]$. The likelihood function generating extrapolation results is a $3$-layer $1\times 1$ convolution having $128$ channels. 
\end{itemize}

\subsection{Training and Evaluation Procedure}
\label{sec:training}
All parameters are initialized with Xavier normalization~\cite{glorot2010understanding} and optimized by the Adam optimizer~\cite{kingma2014adam} with a learning rate of 10$^{-3}$. We train each model for $150$ epochs. At each iteration, we randomly sample $N-3$ nodes to extrapolate the remaining $3$ nodes, with the time length $T=24$. Please note that the number of target nodes has an impact on the performance of the trained models. We conducted experiments to determine the optimal number of target nodes and found that using $3$ nodes generally resulted in the best performance across all baseline models.
For model evaluation, we use all $N$ context nodes to extrapolate $M$ target nodes and we use rolling extrapolation to recover the first bunch of length $T=24$ and then the second, etc.

\subsection{Cross-Domain Evaluation}
We first learn models using the Beijing dataset and then evaluate their performances on the London dataset. We also report the results of training models on London directly. As the London dataset lacks weather information, we remove this attribute in Beijing during training. The other training procedures remain the same. 
Note that we only investigate the performance of PM2.5 concentration and exclude stations BX1, and HR1 due to their large portion of missing values. This is because, for the London dataset, both PM10 and NO2 have a significant amount of missing data (5/7 stations without any signal, 2/1 stations with missing rates larger than 60\%), which makes training unstable and the performance of the models largely depends on the training and testing data split.

\subsection{Evaluation Metrics}
\label{sec:metrics}
We use the rooted mean squared error (RMSE), the mean absolute error (MAE), and the mean absolute percentage error (MAPE) to evaluate the performances of our model and baselines which can be formulated as:
\begin{itemize}
    \item\begin{equation}
        \operatorname{RMSE}=\sqrt{\frac{1}{M} \sum_{m=1}^{M}\left(Y_{m}-\hat{Y}_m\right)^{2}},
    \end{equation}
        \item\begin{equation}
        \operatorname{MAE}=\frac{1}{M} \sum_{m=1}^{M}\left|Y_{i}-\hat{Y}_i\right|,
    \end{equation}
        \item\begin{equation}
        \operatorname{MAPE}= \frac{100\%}{M}\sum_{m=1}^M\frac{|Y_m-\hat{Y}_m|}{{Y}_i},
    \end{equation}
\end{itemize}
where $Y_m$ is the truth node data and $\hat{Y}_m$ is the extrapolations.
\section{Additional Visualization Results}
\label{sec:vis}
We provide more visualization results of STGNP and baselines on stations of the Beijing Dataset. 

\begin{figure*}[!h]
  \centering
  \includegraphics[width=1\linewidth]{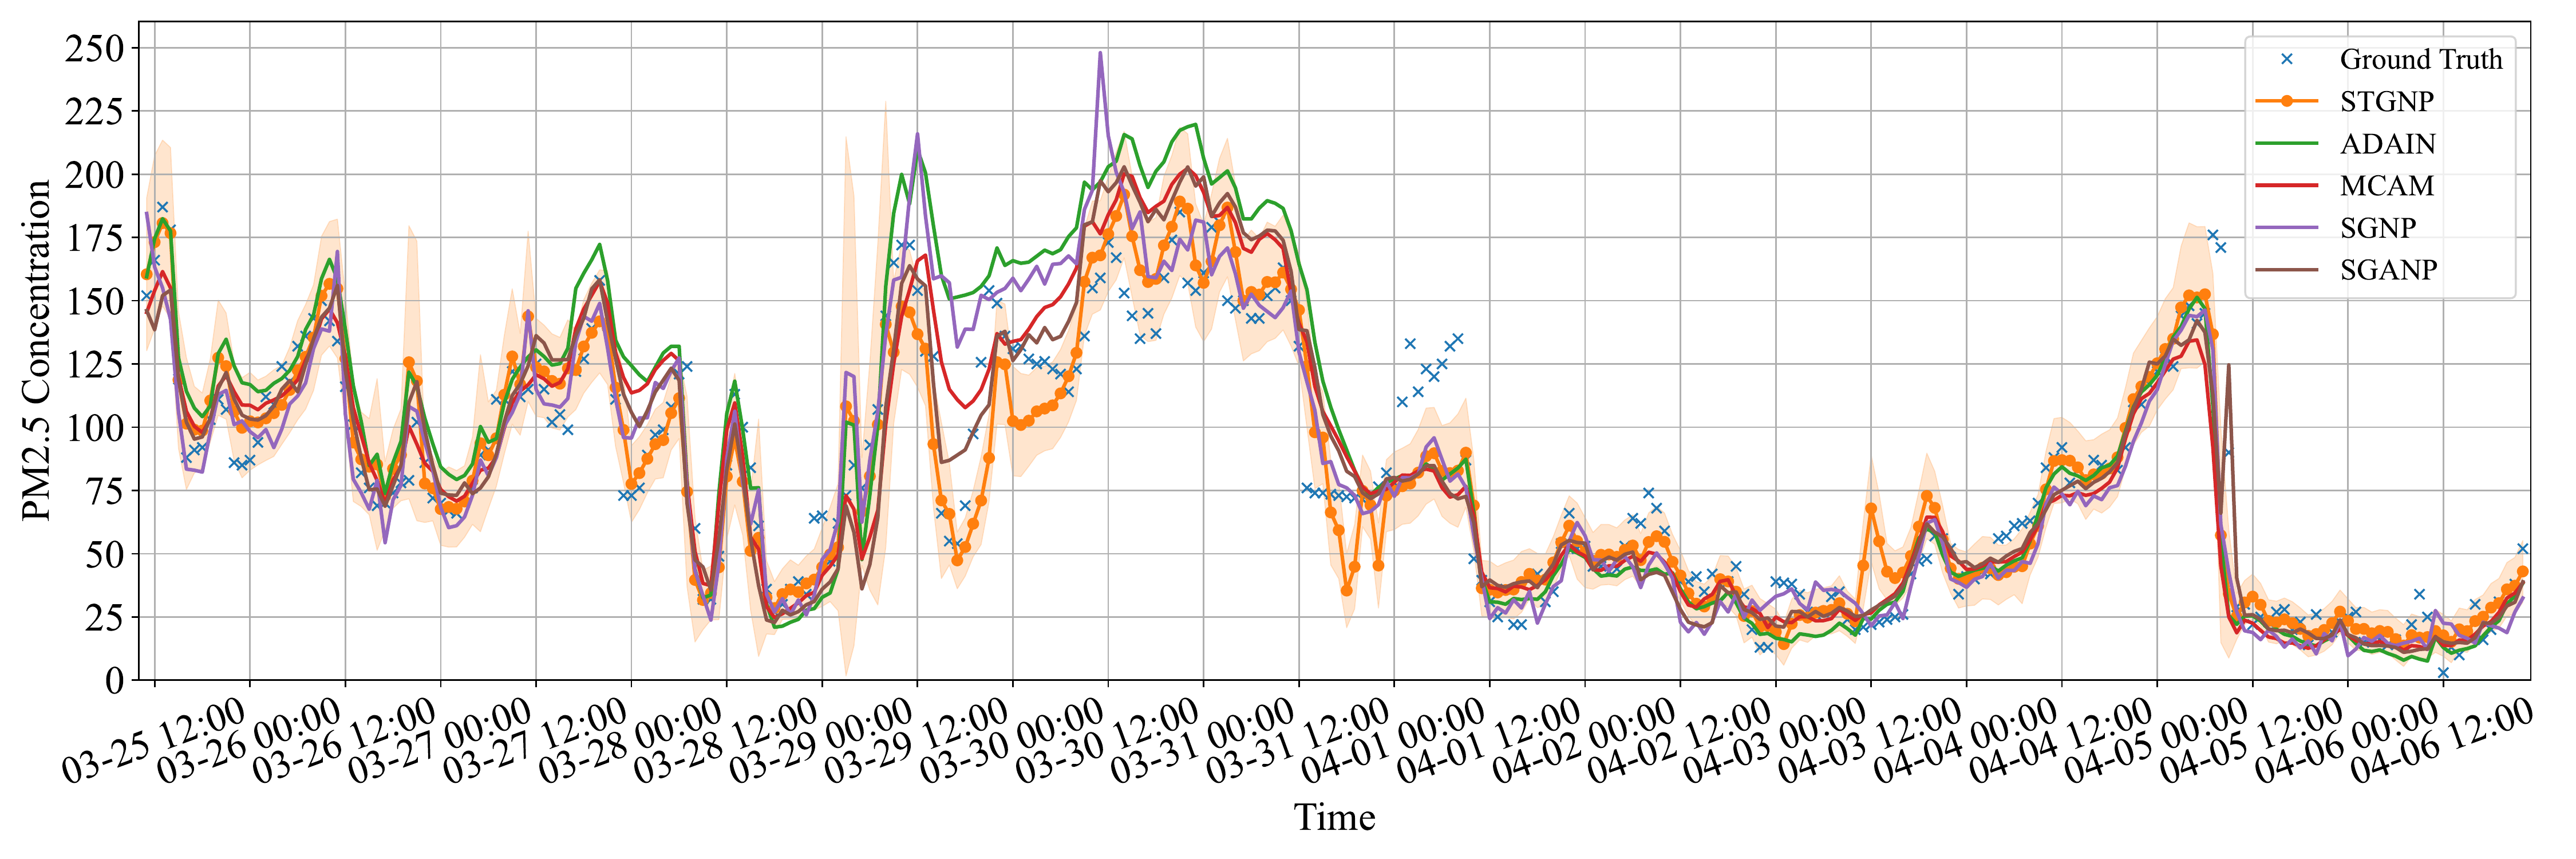}
  \caption{PM2.5 extrapolation performances of the station 1015.}
\end{figure*}

\begin{figure*}[!h]
  \centering
  \includegraphics[width=1\linewidth]{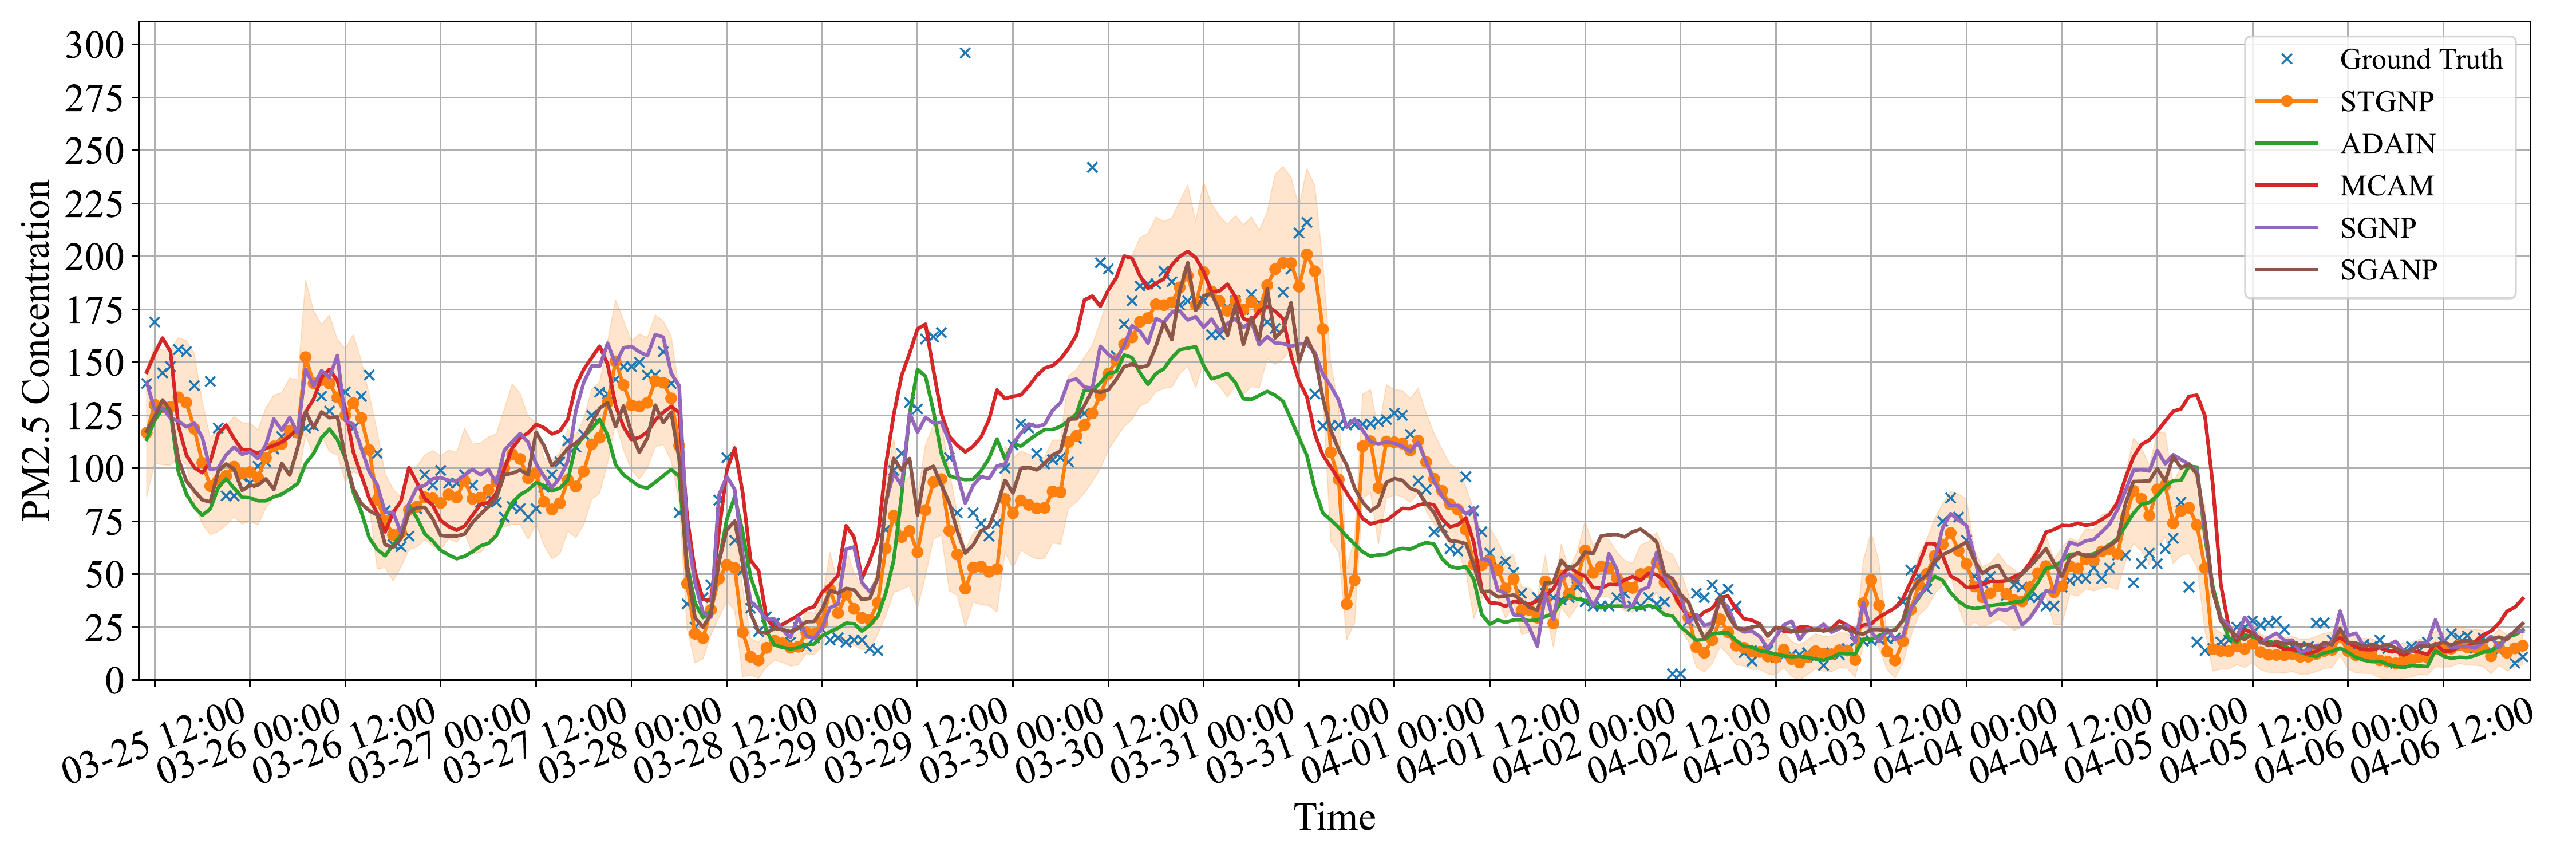}
  \caption{PM2.5 extrapolation performances of the station 1019.}
\end{figure*}

\begin{figure*}[!h]
  \centering
  \includegraphics[width=1\linewidth]{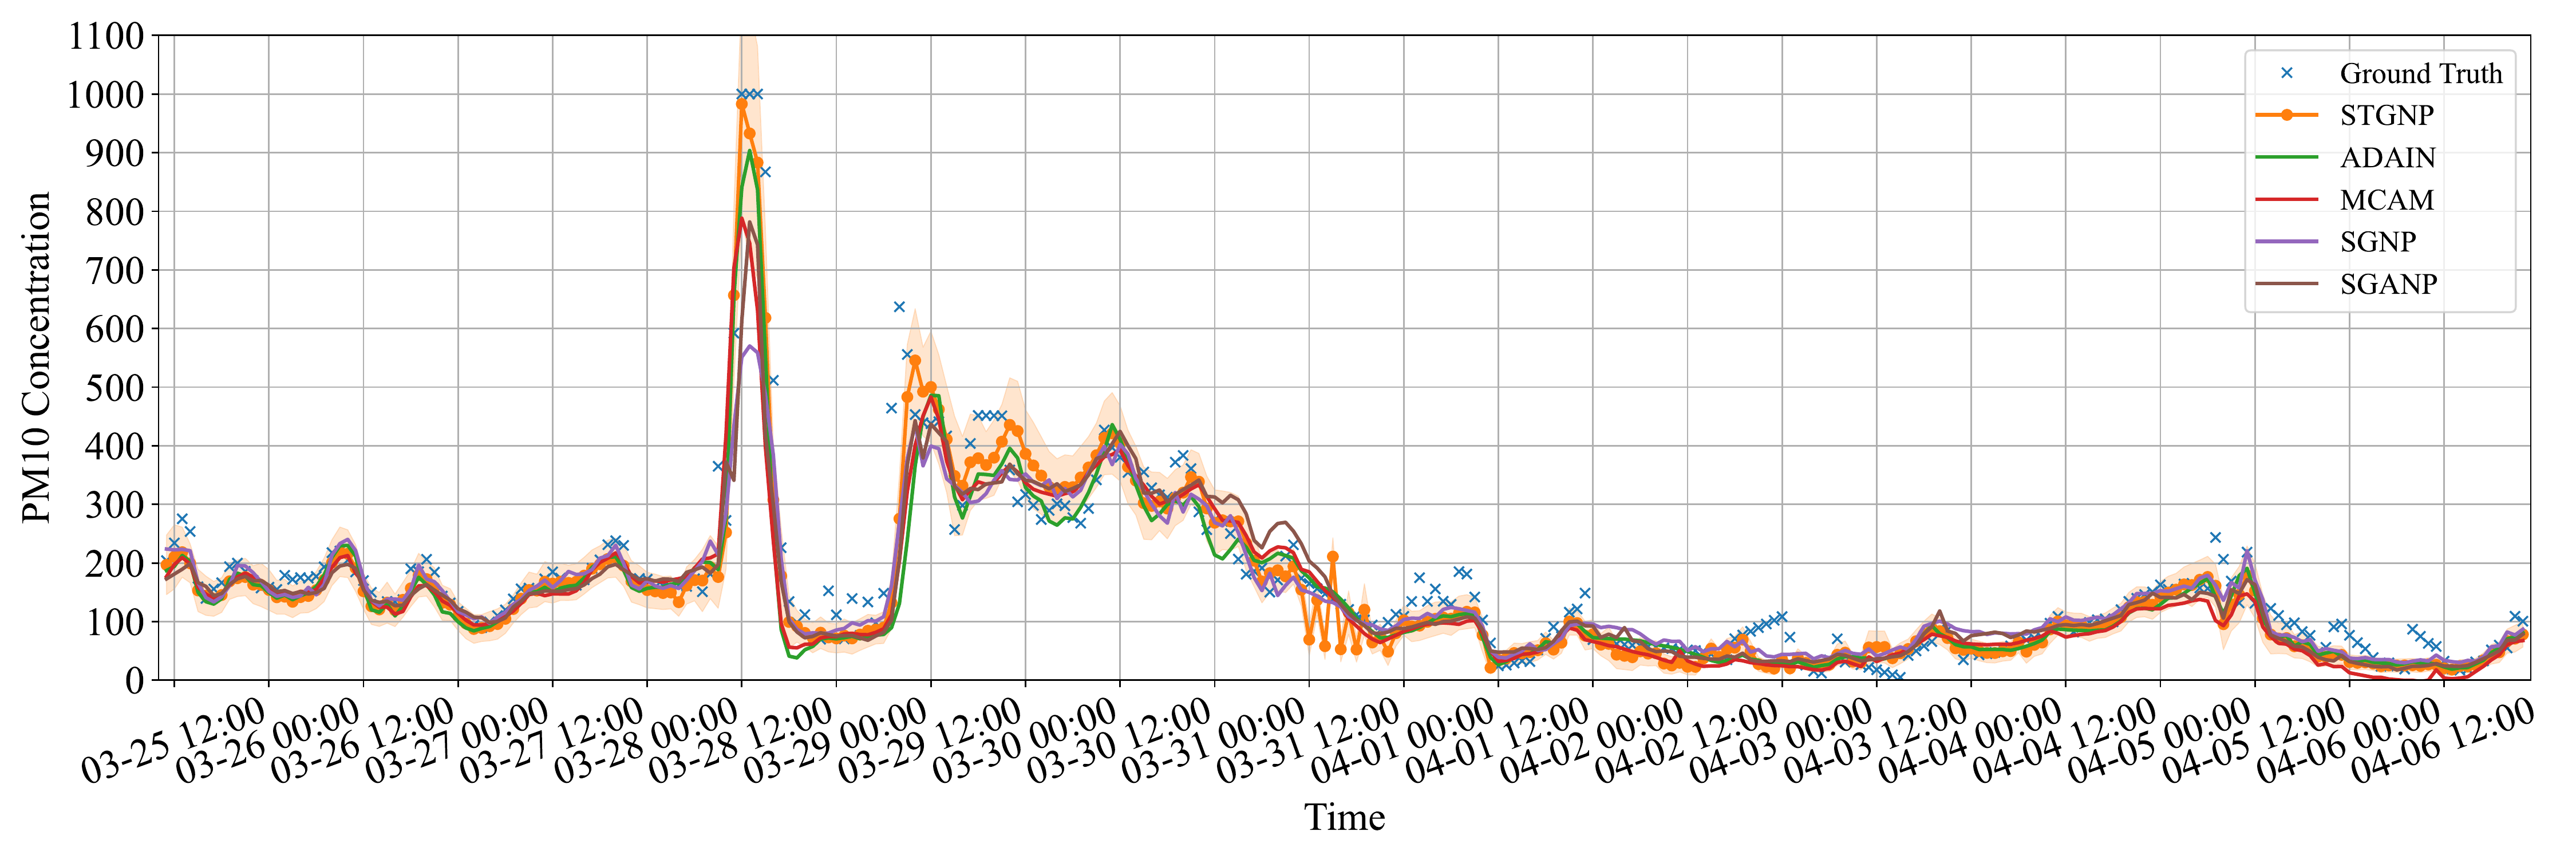}
  \caption{PM10 extrapolation performances of the station 1015.}
\end{figure*}

\begin{figure*}[!h]
  \centering
  \includegraphics[width=1\linewidth]{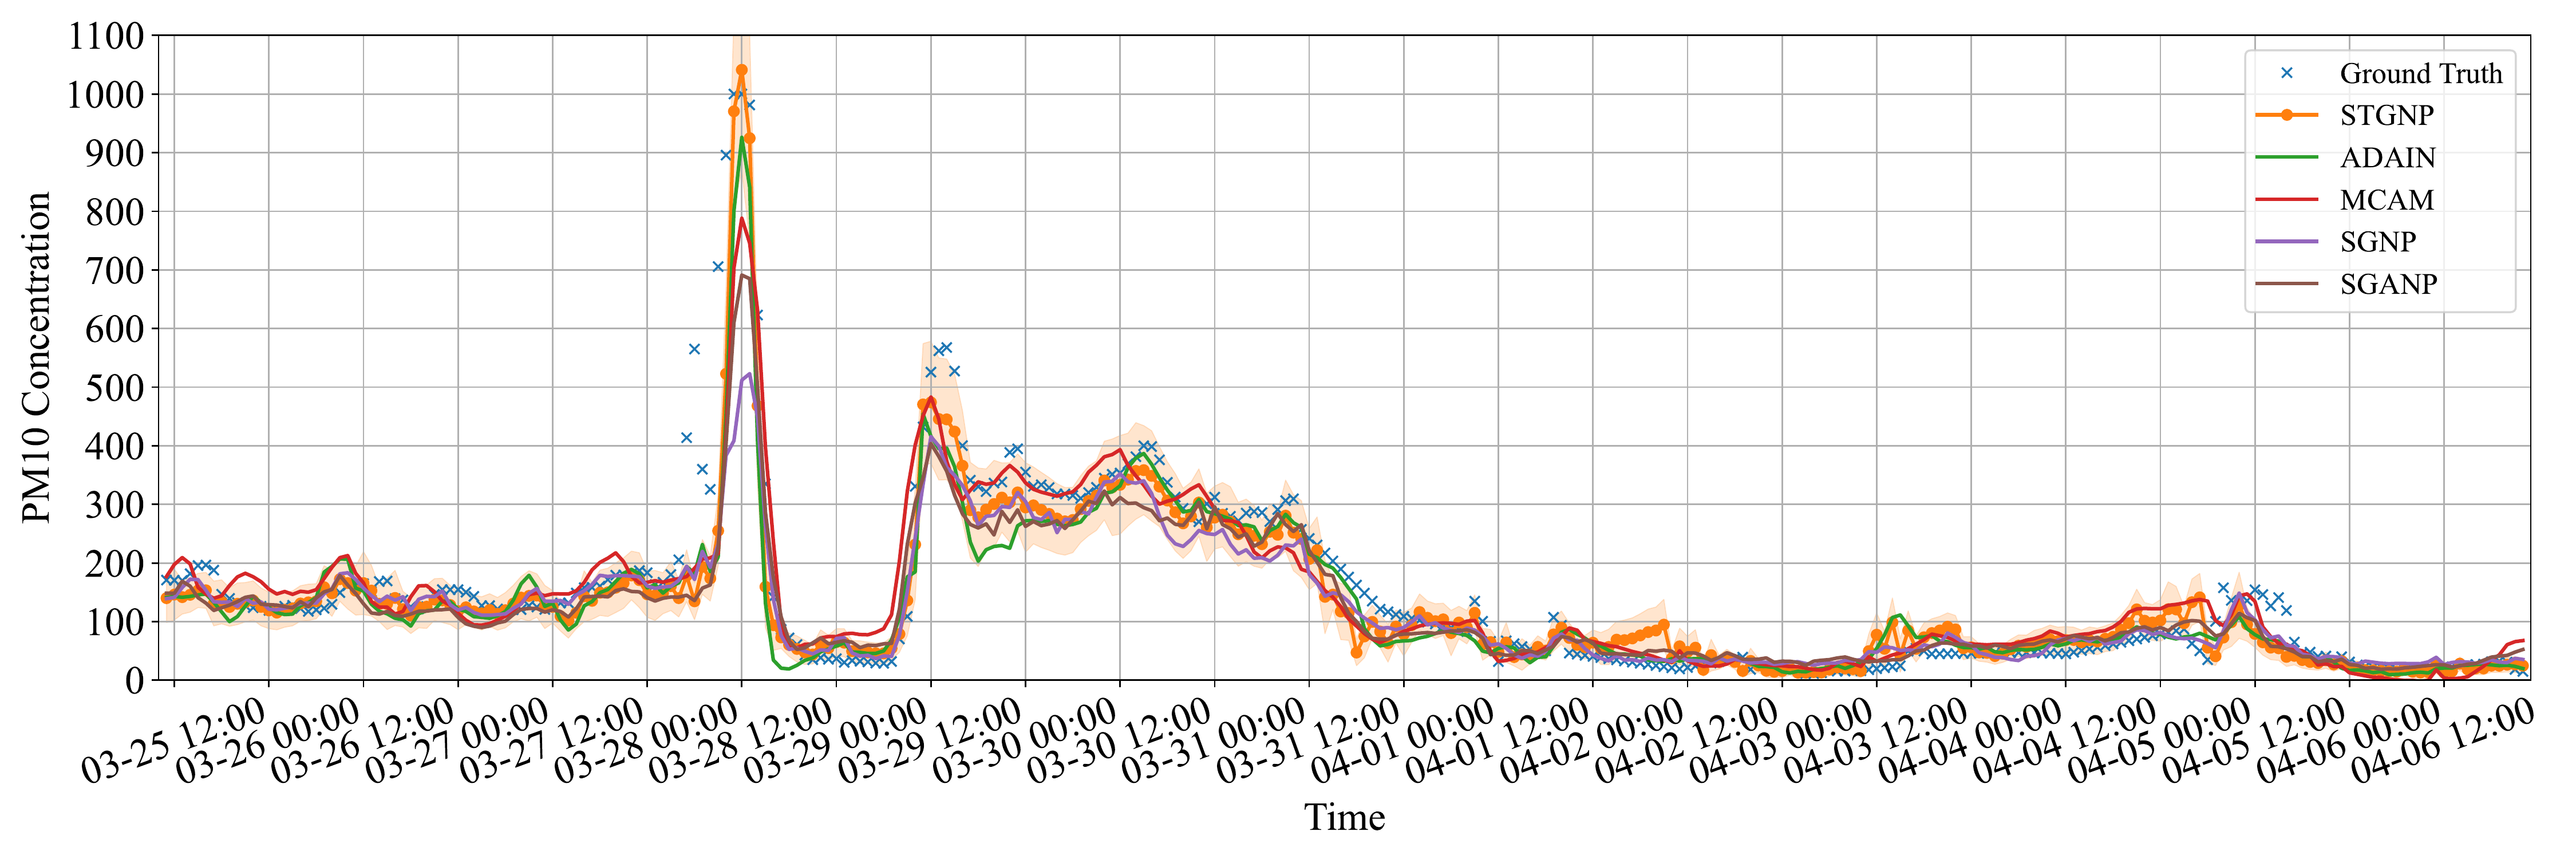}
  \caption{PM10 extrapolation performances of the station 1019.}
\end{figure*}

\begin{figure*}[!h]
  \centering
  \includegraphics[width=1\linewidth]{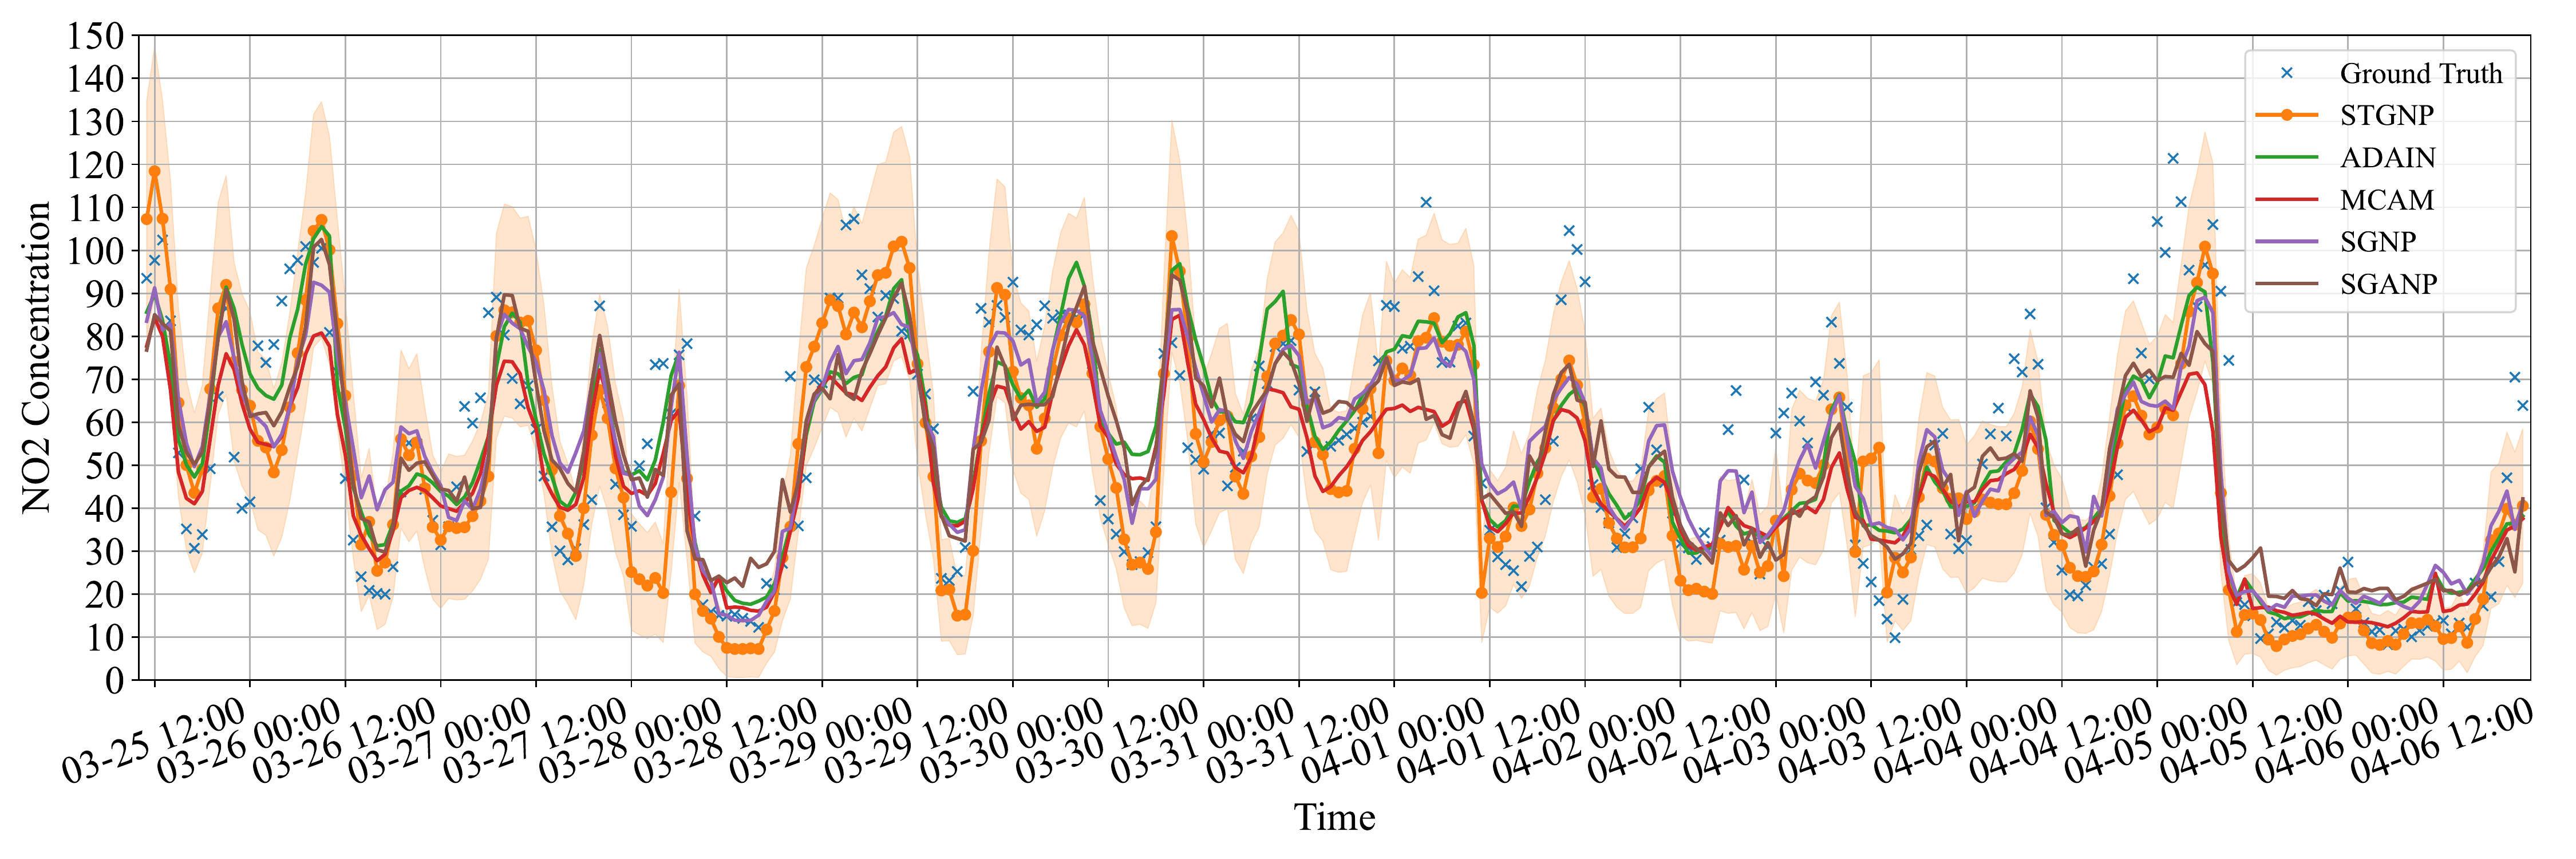}
  \caption{NO2 extrapolation performances of the station 1015.}
\end{figure*}

\begin{figure*}[!h]
  \centering
  \includegraphics[width=1\linewidth]{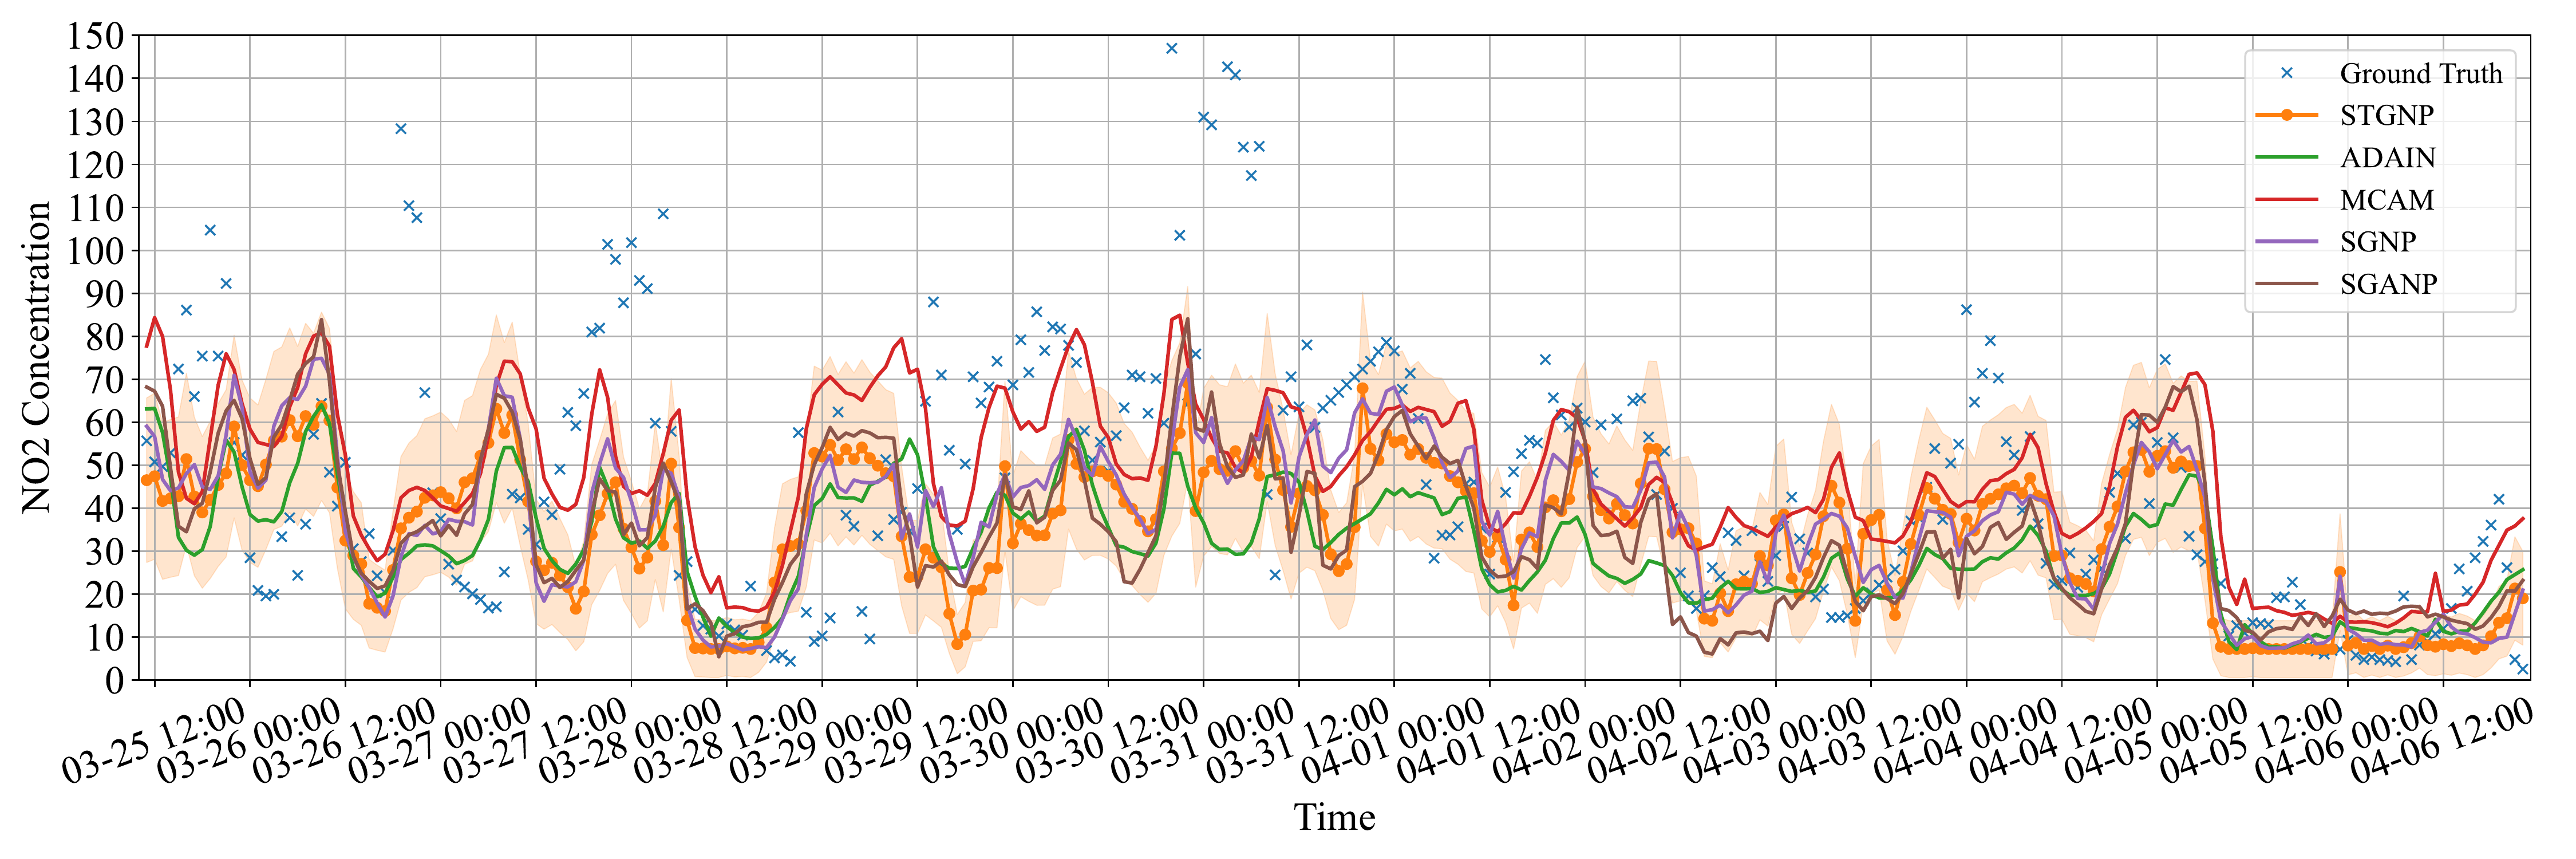}
  \caption{NO2 extrapolation performances of the station 1019.}
\end{figure*}

\begin{figure*}
  \centering
  \includegraphics[width=0.65\linewidth]{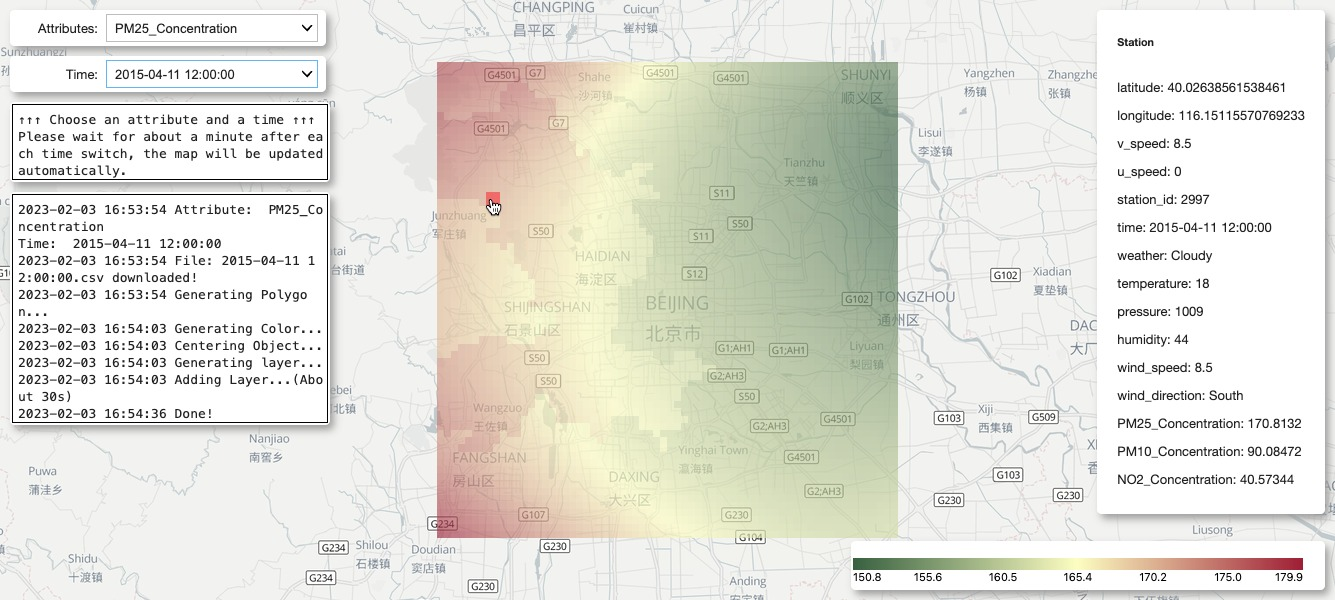}
  \caption{PM2.5 extrapolations.}
  \label{fig:webvis1}
\end{figure*}

\begin{figure*}
  \centering
  \includegraphics[width=0.65\linewidth]{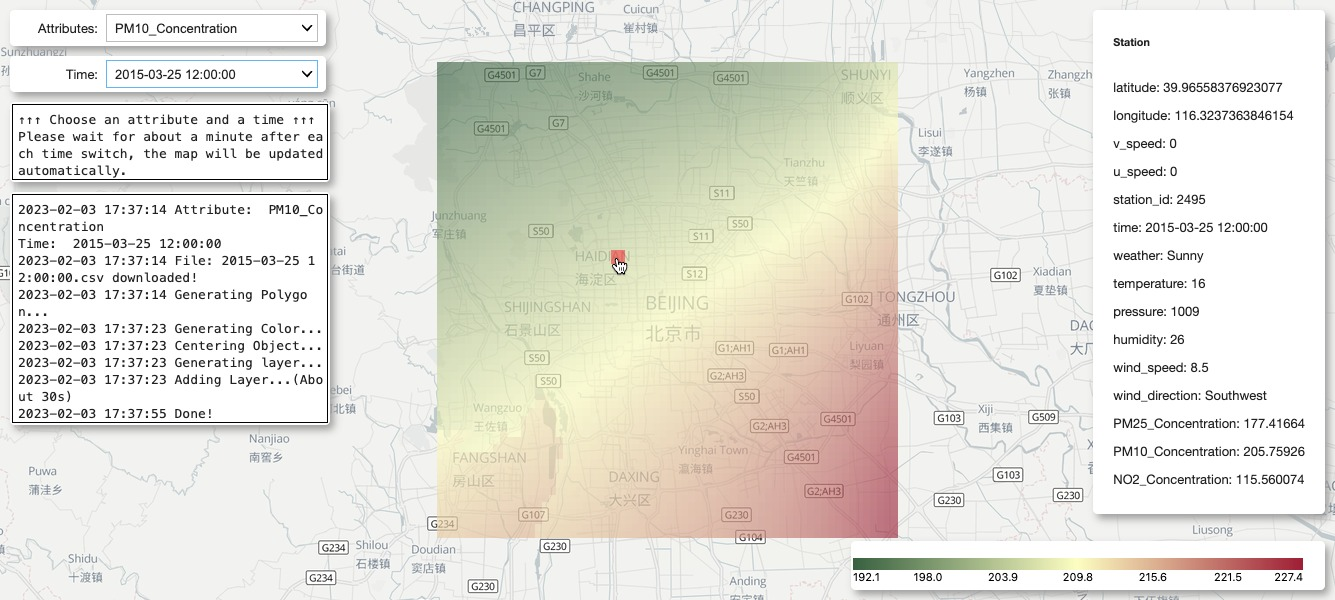}
  \caption{PM2.5 extrapolations.}
  \label{fig:webvis2}
\end{figure*}

\begin{figure*}
  \centering
  \includegraphics[width=0.65\linewidth]{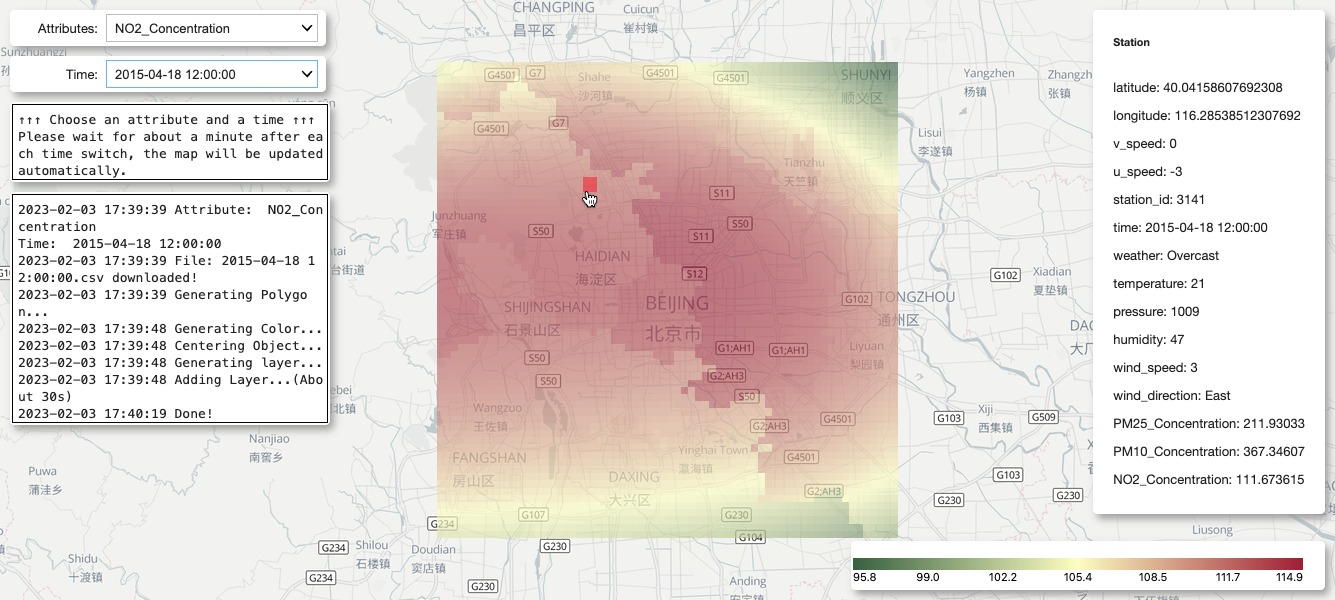}
  \caption{PM10 extrapolations.}
  \label{fig:webvis3}
\end{figure*}

\section{Interactive System}
\label{sec:web}
Being able to visualize extrapolations of different parts of a city allows researchers to understand and analyze data intuitively, which helps decision-making. To facilitate this effect, we developed a cloud-based interactive website where our STGNP is utilized to extrapolate data. Figure~\ref{fig:webvis1}-\ref{fig:webvis3} illustrate the system's interface, where users can select the attribute and time of extrapolations to be visualized from the top left corner. The user can also click any region on the map to read the numerical results of extrapolations and other covariates as shown on the right side. The website is anonymously accessible at {\color{blue}\url{https://stgnp.tech}}. Currently, the loading speed is slow. Please clear the cache if the website fails to load.
